# Supplementary material for: Riemann correlator in de Sitter including loop corrections from conformal fields
Source: arXiv:1403.3335 source file (2014-07-31)
Supplement: Supplementary file 1 [file appendix_curvature.tex]

To facilitate comparison with other results, here we express our result also in terms of other maximally symmetric bitensors. Especially, we want to give in in terms of the normal vector $n_a$ and $n_{a'}$ to the geodesic connecting the two points (if it exists) and the parallel propagator $\tilde{g}_{ab'}$. However, as those become singular as one of the points lies on the lightcone of the other or its antipodal point, which is the limit $Z \to \pm1$, they are not suitable for the study of this limit. However, because of their normalization they are advantegeous to study the behaviour in the limit of large time- and space-like separations, $Z \to \pm\infty$.

Using then the formulae \eqref{relation_z_n} which relates them to the derivatives of $Z$, we get
\begin{equation}
\label{weyl_correlator_normal}
\begin{split}
\expect{{\tilde{C}^{ab}}{}_{cd} {\tilde{C}^{m'n'}}{}_{p'q'}} &= \frac{4 \kappa^2 H^6}{\mathpi^2} \sum_{k=1}^9 {}^{(k)}\mathcal{N}^{[ab]}{}_{[cd]}{}^{[m'n']}{}_{[p'q']} \times \\
&\quad\times \bigg[ \left( 1 + 6 \alpha \kappa^2 H^2 \left( \ln\left( \frac{\mu}{H} \right) + \gamma \right) - \left( 5 \alpha - 2 \beta \right) \kappa^2 H^2 \right) \mathcal{N}^{(0,k)} + \frac{3}{2} \alpha \kappa^2 H^2 \mathcal{N}^{(1,k)} \bigg] \eqend{,}
\end{split}
\end{equation}
where
\begin{equation}
\begin{split}
{}^{(1)}\mathcal{N}^{ab}{}_{cd}{}^{m'n'}{}_{p'q'} &= \delta^a_c \delta^b_d \delta^{m'}_{p'} \delta^{n'}_{q'} \\
{}^{(2)}\mathcal{N}^{ab}{}_{cd}{}^{m'n'}{}_{p'q'} &= \delta^a_c \delta^{m'}_{p'} \left( n^b n_d \delta^{n'}_{q'} + \delta^b_d n^{n'} n_{q'} \right) \\
{}^{(3)}\mathcal{N}^{ab}{}_{cd}{}^{m'n'}{}_{p'q'} &= \delta^a_c \delta^{m'}_{p'} n^b n_d n^{n'} n_{q'} \\
{}^{(4)}\mathcal{N}^{ab}{}_{cd}{}^{m'n'}{}_{p'q'} &= \delta^a_c \delta^{m'}_{p'} \left( n^b \tilde{g}_d^{n'} n_{q'} + n_d \tilde{g}^{bn'} n_{q'} + n^b \tilde{g}_{dq'} n^{n'} + n_d \tilde{g}^b_{q'} n^{n'} \right) \\
{}^{(5)}\mathcal{N}^{ab}{}_{cd}{}^{m'n'}{}_{p'q'} &= \delta^a_c \delta^{m'}_{p'} \left( \tilde{g}^{bn'} \tilde{g}_{dq'} + \tilde{g}^b_{q'} \tilde{g}_{dn'} \right) \\
{}^{(6)}\mathcal{N}^{ab}{}_{cd}{}^{m'n'}{}_{p'q'} &= \left( \delta^a_c n^{m'} n_{p'} + n^a n_c \delta^{m'}_{p'} \right) \left( \tilde{g}^{bn'} \tilde{g}_{dq'} + \tilde{g}^b_{q'} \tilde{g}_d^{n'} \right) \\
{}^{(7)}\mathcal{N}^{ab}{}_{cd}{}^{m'n'}{}_{p'q'} &= n^a n_c n^{m'} n_{p'} \left( \tilde{g}^{bn'} \tilde{g}_{dq'} + \tilde{g}^b_{q'} \tilde{g}_d^{n'} \right) \\
{}^{(8)}\mathcal{N}^{ab}{}_{cd}{}^{m'n'}{}_{p'q'} &= \left( n^a \tilde{g}_c^{m'} n_{p'} + n_c \tilde{g}^{am'} n_{p'} + n^a \tilde{g}_{cp'} n^{m'} + n_c \tilde{g}^a_{p'} n^{m'} \right) \left( \tilde{g}^{bn'} \tilde{g}_{dq'} + \tilde{g}^{b}_{q'} \tilde{g}_d^{n'} \right) \\
{}^{(9)}\mathcal{N}^{ab}{}_{cd}{}^{m'n'}{}_{p'q'} &= \left( \tilde{g}^{am'} \tilde{g}_{cp'} + \tilde{g}^a_{p'} \tilde{g}_c^{m'} \right) \left( \tilde{g}^{bn'} \tilde{g}_{dq'} + \tilde{g}^b_{q'} \tilde{g}_d^{n'} \right) \eqend{,}
\end{split}
\end{equation}
\begin{equation}
\begin{split}
\mathcal{N}^{(0,1)} &= - \frac{1}{6} \mathcal{N}^{(0,7)} + \mathcal{N}^{(0,8)} + \mathcal{N}^{(0,9)} \\
\mathcal{N}^{(0,2)} &= \frac{1}{2} \mathcal{N}^{(0,7)} - 3 \mathcal{N}^{(0,8)} \\
\mathcal{N}^{(0,3)} &= - \mathcal{N}^{(0,7)} \\
\mathcal{N}^{(0,4)} &= \frac{1}{4} \mathcal{N}^{(0,7)} - 3 \mathcal{N}^{(0,8)} \\
\mathcal{N}^{(0,5)} &= \frac{1}{4} \mathcal{N}^{(0,7)} - \frac{3}{2} \mathcal{N}^{(0,8)} - 3 \mathcal{N}^{(0,9)} \\
\mathcal{N}^{(0,6)} &= - \frac{1}{2} \mathcal{N}^{(0,7)} + 3 \mathcal{N}^{(0,8)} \\
\mathcal{N}^{(0,7)} &= 12 (1 - Z + \mathi \sgneps)^{-3} \\
\mathcal{N}^{(0,8)} &= \frac{1}{4} (7-Z) (1 - Z + \mathi \sgneps)^{-3} \\
\mathcal{N}^{(0,9)} &= \frac{1}{8} (3-Z) (1 - Z + \mathi \sgneps)^{-3} \eqend{,}
\end{split}
\end{equation}
and
\begin{equation}
\begin{split}
\mathcal{N}^{(1,1)} &= - \frac{1}{6} \mathcal{N}^{(1,7)} + \mathcal{N}^{(1,8)} + \mathcal{N}^{(1,9)} \\
\mathcal{N}^{(1,2)} &= \frac{1}{2} \mathcal{N}^{(1,7)} - 3 \mathcal{N}^{(1,8)} \\
\mathcal{N}^{(1,3)} &= - \mathcal{N}^{(1,7)} \\
\mathcal{N}^{(1,4)} &= \frac{1}{4} \mathcal{N}^{(1,7)} - 3 \mathcal{N}^{(1,8)} \\
\mathcal{N}^{(1,5)} &= \frac{1}{4} \mathcal{N}^{(1,7)} - \frac{3}{2} \mathcal{N}^{(1,8)} - 3 \mathcal{N}^{(1,9)} \\
\mathcal{N}^{(1,6)} &= - \frac{1}{2} \mathcal{N}^{(1,7)} + 3 \mathcal{N}^{(1,8)} \\
\mathcal{N}^{(1,7)} &= 24 (1 - Z - \mathi \epsilon)^{-3} \ln\left[ \frac{1}{2} (1 - Z + \mathi \sgneps) \right] + 10 (7 + 5 Z) (1 - Z + \mathi \sgneps)^{-4} \\
&= - (1 + Z)^3 (1 - Z - \mathi \epsilon)^{-3} \hypergeom{2}{1}\left[ 3, 3; 4; \frac{1}{2} (1 + Z - \mathi \sgneps) \right] + (58 + 4 Z - 14 Z^2) (1 - Z - \mathi \epsilon)^{-5} \\
\mathcal{N}^{(1,8)} &= 4 (1 + 2 Z + 3 Z^2) (1 + Z + \mathi \epsilon)^{-3} (1 - Z - \mathi \epsilon)^{-3} \ln\left[ \frac{1}{2} (1 - Z + \mathi \sgneps) \right] \\
&\qquad+ (9 + 20 Z + 19 Z^2) (1 + Z + \mathi \epsilon)^{-2} (1 - Z + \mathi \sgneps)^{-4} \\
&= - \frac{1}{6} (1 + 2 Z + 3 Z^2) (1 - Z - \mathi \epsilon)^{-3} \hypergeom{2}{1}\left[ 3, 3; 4; \frac{1}{2} (1 + Z - \mathi \sgneps) \right] + (7 - Z) (1 - Z - \mathi \epsilon)^{-5} \\
\mathcal{N}^{(1,9)} &= 4 Z (1 + Z + \mathi \epsilon)^{-3} (1 - Z - \mathi \epsilon)^{-3} \ln\left[ \frac{1}{2} (1 - Z + \mathi \sgneps) \right] \\
&\qquad+ (1 + 5 Z) (1 + Z + \mathi \epsilon)^{-2} (1 - Z + \mathi \sgneps)^{-4} \\
&= - \frac{1}{6} Z (1 - Z - \mathi \epsilon)^{-3} \hypergeom{2}{1}\left[ 3, 3; 4; \frac{1}{2} (1 + Z - \mathi \sgneps) \right] + (1 - Z - \mathi \epsilon)^{-5} \eqend{.}
\end{split}
\end{equation}
The fact that there are only three independent scalar coefficients which contribute to the \person{Weyl}-\person{Weyl} correlation function (which is not true for the \person{Riemann}-\person{Riemann} correlation function) is a simple consequence of the tracelessness of the \person{Weyl} tensor. Namely, for a \person{de Sitter}-invariant bitensor, there are only three combinations of invariant bitensors which have vanishing trace on any contraction, which are
\begin{equation}
\begin{split}
&\left[ - 2 {}^{(1)}\mathcal{N} + 6 {}^{(2)}\mathcal{N} - 12 {}^{(3)}\mathcal{N} + 3 {}^{(4)}\mathcal{N} + 3 {}^{(5)}\mathcal{N} - 6 {}^{(6)}\mathcal{N} + 12 {}^{(7)}\mathcal{N} \right]{}^{[ab]}{}_{[cd]}{}^{[m'n']}{}_{[p'q']} \eqend{,}\\
&\left[ - 12 {}^{(3)}\mathcal{N} - 3 {}^{(4)}\mathcal{N} + 12 {}^{(7)}\mathcal{N} + 2 {}^{(8)}\mathcal{N} \right] {}^{[ab]}{}_{[cd]}{}^{[m'n']}{}_{[p'q']} \eqend{,}\\
&\left[ {}^{(1)}\mathcal{N} - 3 {}^{(5)}\mathcal{N} + {}^{(9)}\mathcal{N} \right] {}^{[ab]}{}_{[cd]}{}^{[m'n']}{}_{[p'q']} \eqend{.}
\end{split}
\end{equation}
The same observation of course also applies to the expression of the \person{Weyl}-\person{Weyl} correlation function using derivatives of $Z$ as the basic bitensors \eqref{weyl_correlator}, although there the corresponding expressions involve polynomials of $Z$ instead of only numeric factors owing to the non-normalization of those bitensors.

% {}^{(1)}\mathcal{R}^{ab}{}_{cd}{}^{m'n'}{}_{p'q'} = {}^{(1)}\mathcal{N}^{ab}{}_{cd}{}^{m'n'}{}_{p'q'}
% {}^{(2)}\mathcal{R}^{ab}{}_{cd}{}^{m'n'}{}_{p'q'} = (1-Z^2) {}^{(2)}\mathcal{N}^{ab}{}_{cd}{}^{m'n'}{}_{p'q'}
% {}^{(3)}\mathcal{R}^{ab}{}_{cd}{}^{m'n'}{}_{p'q'} = (1-Z^2)^2 {}^{(3)}\mathcal{N}^{ab}{}_{cd}{}^{m'n'}{}_{p'q'}
% {}^{(4)}\mathcal{R}^{ab}{}_{cd}{}^{m'n'}{}_{p'q'} = (1-Z^2) {}^{(4)}\mathcal{N}^{ab}{}_{cd}{}^{m'n'}{}_{p'q'} + 4 (1-Z^2) (1-Z) {}^{(3)}\mathcal{N}^{ab}{}_{cd}{}^{m'n'}{}_{p'q'}
% {}^{(5)}\mathcal{R}^{ab}{}_{cd}{}^{m'n'}{}_{p'q'} = {}^{(5)}\mathcal{N}^{ab}{}_{cd}{}^{m'n'}{}_{p'q'} + (1-Z) {}^{(4)}\mathcal{N}^{ab}{}_{cd}{}^{m'n'}{}_{p'q'} + 2 (1-Z)^2 {}^{(3)}\mathcal{N}^{ab}{}_{cd}{}^{m'n'}{}_{p'q'}
% {}^{(6)}\mathcal{R}^{ab}{}_{cd}{}^{m'n'}{}_{p'q'} = (1-Z^2) {}^{(6)}\mathcal{N}^{ab}{}_{cd}{}^{m'n'}{}_{p'q'}
% {}^{(7)}\mathcal{R}^{ab}{}_{cd}{}^{m'n'}{}_{p'q'} = (1-Z^2)^2 {}^{(7)}\mathcal{N}^{ab}{}_{cd}{}^{m'n'}{}_{p'q'}
% {}^{(8)}\mathcal{R}^{ab}{}_{cd}{}^{m'n'}{}_{p'q'} = (1-Z^2) {}^{(8)}\mathcal{N}^{ab}{}_{cd}{}^{m'n'}{}_{p'q'} + 6 (1-Z^2) (1-Z) {}^{(7)}\mathcal{N}^{ab}{}_{cd}{}^{m'n'}{}_{p'q'}
% {}^{(9)}\mathcal{R}^{ab}{}_{cd}{}^{m'n'}{}_{p'q'} = {}^{(9)}\mathcal{N}^{ab}{}_{cd}{}^{m'n'}{}_{p'q'} + 2 (1-Z) {}^{(8)}\mathcal{N}^{ab}{}_{cd}{}^{m'n'}{}_{p'q'} + 6 (1-Z)^2 {}^{(7)}\mathcal{N}^{ab}{}_{cd}{}^{m'n'}{}_{p'q'}

Furthermore, for the \person{Ricci}-\person{Ricci} correlation function \eqref{ricci_correlator} we get in the same way
\begin{equation}
\label{ricci_correlator_normal}
\begin{split}
\expect{{\tilde{R}^b}{}_d {\tilde{R}^{n'}}{}_{q'}} &= \frac{15 \alpha \kappa^4 H^8}{4 \mathpi^2} \bigg[ - \delta^b_d \delta^{n'}_{q'} + 16 n^b n_d n^{n'} n_{q'} + 2 \left( \tilde{g}^{;bn'} \tilde{g}_{;dq'} + \tilde{g}^{;b}_{;q'} \tilde{g}_{;d}^{;n'} \right) \\
&\qquad\qquad\qquad+ 4 \left( n_b \tilde{g}_{;d}^{;n'} n_{q'} + n_d \tilde{g}^{;bn'} n_{q'} + n^b \tilde{g}_{;dq'} n^{n'} + n_d \tilde{g}^{;b}_{;q'} n^{n'} \right) \bigg] (1 - Z + \mathi \sgneps)^{-4} \eqend{,}
\end{split}
\end{equation}
as well as for the \person{Ricci}-\person{Weyl} correlation function \eqref{ricciweyl_correlator}
\begin{equation}
\label{ricciweyl_correlator_normal}
\begin{split}
\expect{{\tilde{R}^b}{}_d {\tilde{C}^{m'n'}}{}_{p'q'}} &= \frac{3 \alpha \kappa^4 H^8}{\mathpi^2} \bigg[ 2 ( \delta^b_d - n^b n_d ) \delta^{[m'}_{[p'} \delta^{n']}_{q']} \\
&\qquad- 3 \delta^{[m'}_{[p'} \left( n_{q']} \tilde{g}^{;n']b} n_d + n^{n']} \tilde{g}^{;b}_{;q']} n_d + n_{q']} \tilde{g}_{;d}^{;n']} n^b + n^{n']} \tilde{g}_{;q']d} n^b + \tilde{g}^b_{q']} \tilde{g}_d^{n']} + \tilde{g}^{n']b} \tilde{g}_{q']d} \right) \\
&\qquad+ 6 \left( \tilde{g}^b_{[p'} \tilde{g}_d^{[m'} + \tilde{g}^{[m'b} \tilde{g}_{[p'd} - \delta^b_d \delta^{[m'}_{[p'} \right) n^{n']} n_{q']} \bigg] (1+Z) (1 - Z + \mathi \sgneps)^{-4} \eqend{.}
\end{split}
\end{equation}

Note that while in this basis of maximally symmetric bitensors it may seem that the correlation functions are less singular as $Z \to \pm1$, this isn't the case because, as already said before, the basis itself becomes singular in this limit.??? fa falta dir-ho un altre cop?
